# Supplementary material for: Towards High-fidelity 3D Talking Avatar with Personalized Dynamic Texture
Source: arXiv:2503.00495 source file (2025-03-01)
Supplement: Supplementary file 4 [file dataset.tex]

\section{Dataset Details}
